# Supplementary material for: Accurate prediction of structural and mechanical properties on amorphous materials enabled through machine-learning potentials: a case study of silicon nitride
Source: arXiv:2408.05782 source file (2024-08-11)
Supplement: Supplementary file 1 [file a-SiN_elasticity_SI.pdf]

# Supporting Information: Accurate prediction of structural and mechanical properties on amorphous materials enabled through machine-learning potentials: a case study of silicon nitride

Ganesh Kumar Nayak[a,1], Prashanth Srinivasan[c], Juraj Todt[a], Rostislav Daniel[a], Paolo Nicolini[d], David Holec[a]

[a] *Department of Materials Science, Montanuniversität Leoben, Franz-Josef-Strasse 18, A-8700, Leoben, Austria*
[b] *Materials Chemistry, RWTH Aachen University, Kopernikusstraße 10, 52074, Aachen, Germany*
[c] *Department of Materials Design, Institute for Materials Science, University of Stuttgart, Pfaffenwaldring 55, D-70569, Stuttgart, Stuttgart*
[d] *Institute of Physics (FZU), Czech Academy of Sciences, Na Slovance 2, 18200, Prague, Czechia*

*Email addresses:* nayak@mch.rwth-aachen.de (Ganesh Kumar Nayak), david.holec@unileoben.ac.at (David Holec)
*URL:* http://cms.unileoben.ac.at (David Holec)

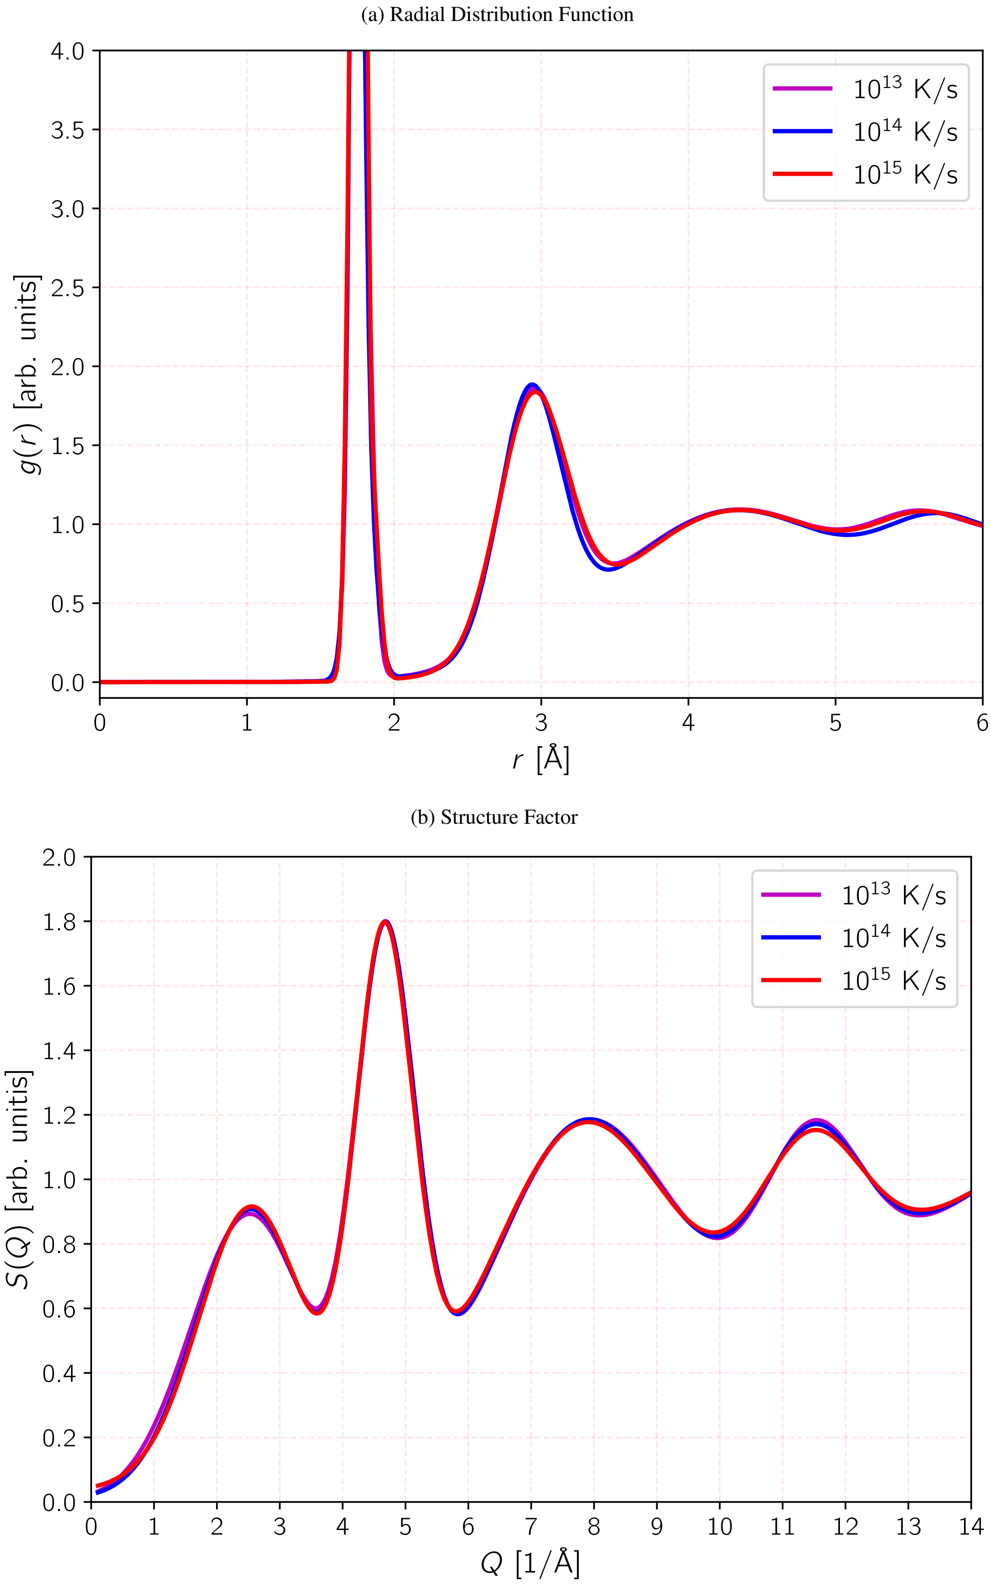


Figure 1: Comparision of (a) the total radial distribution function of a-$Si_3N_4$ and (b) computed structure factor of different quenching rates from the MTP-based molecular dynamics.

(a) Bond Length AIMD 112 atoms vs MTP 7000 atoms

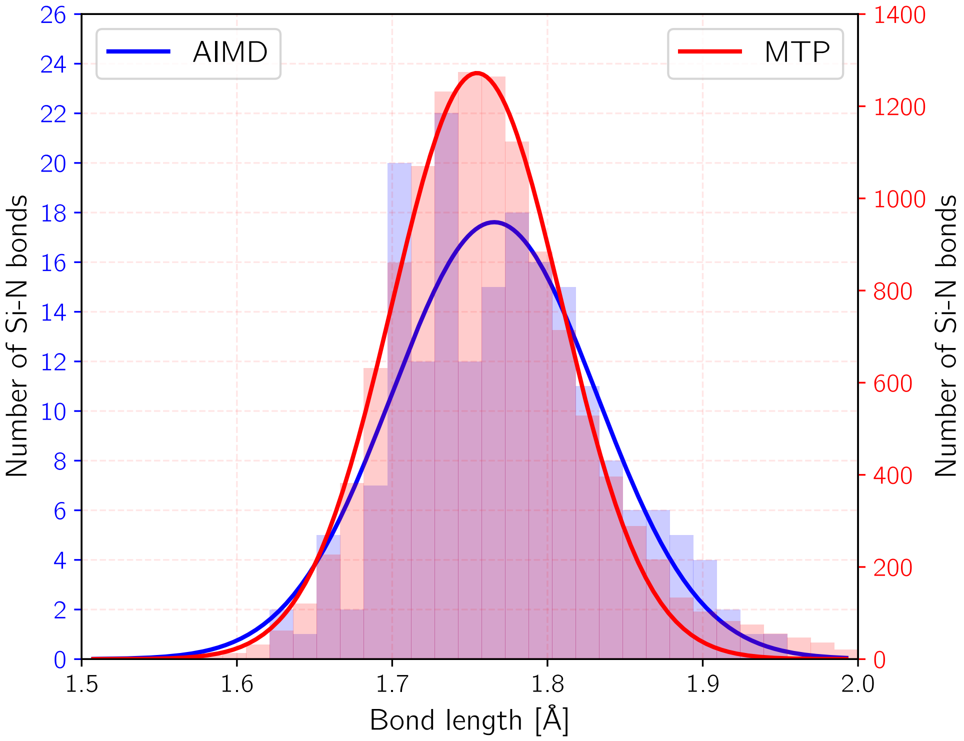


(b) Bond Angle AIMD 112 atoms vs MTP 7000 atoms

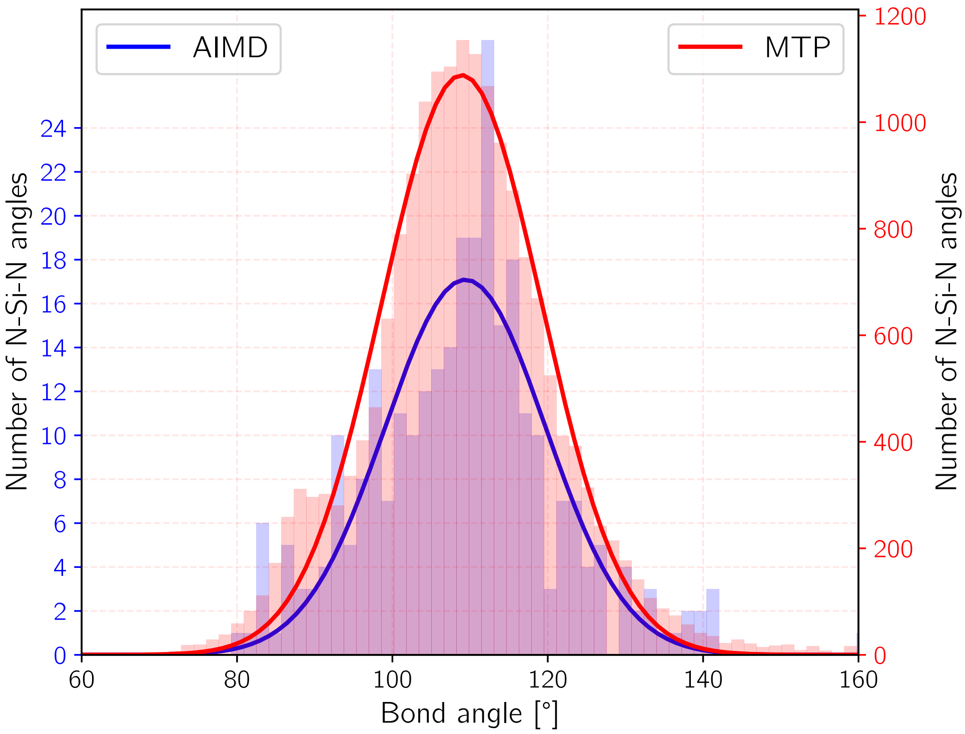


Figure 2: Comparision of (a) bond length distribution and (b) bond angle distribution of AIMD 112 atoms and MTP 7000 atoms.

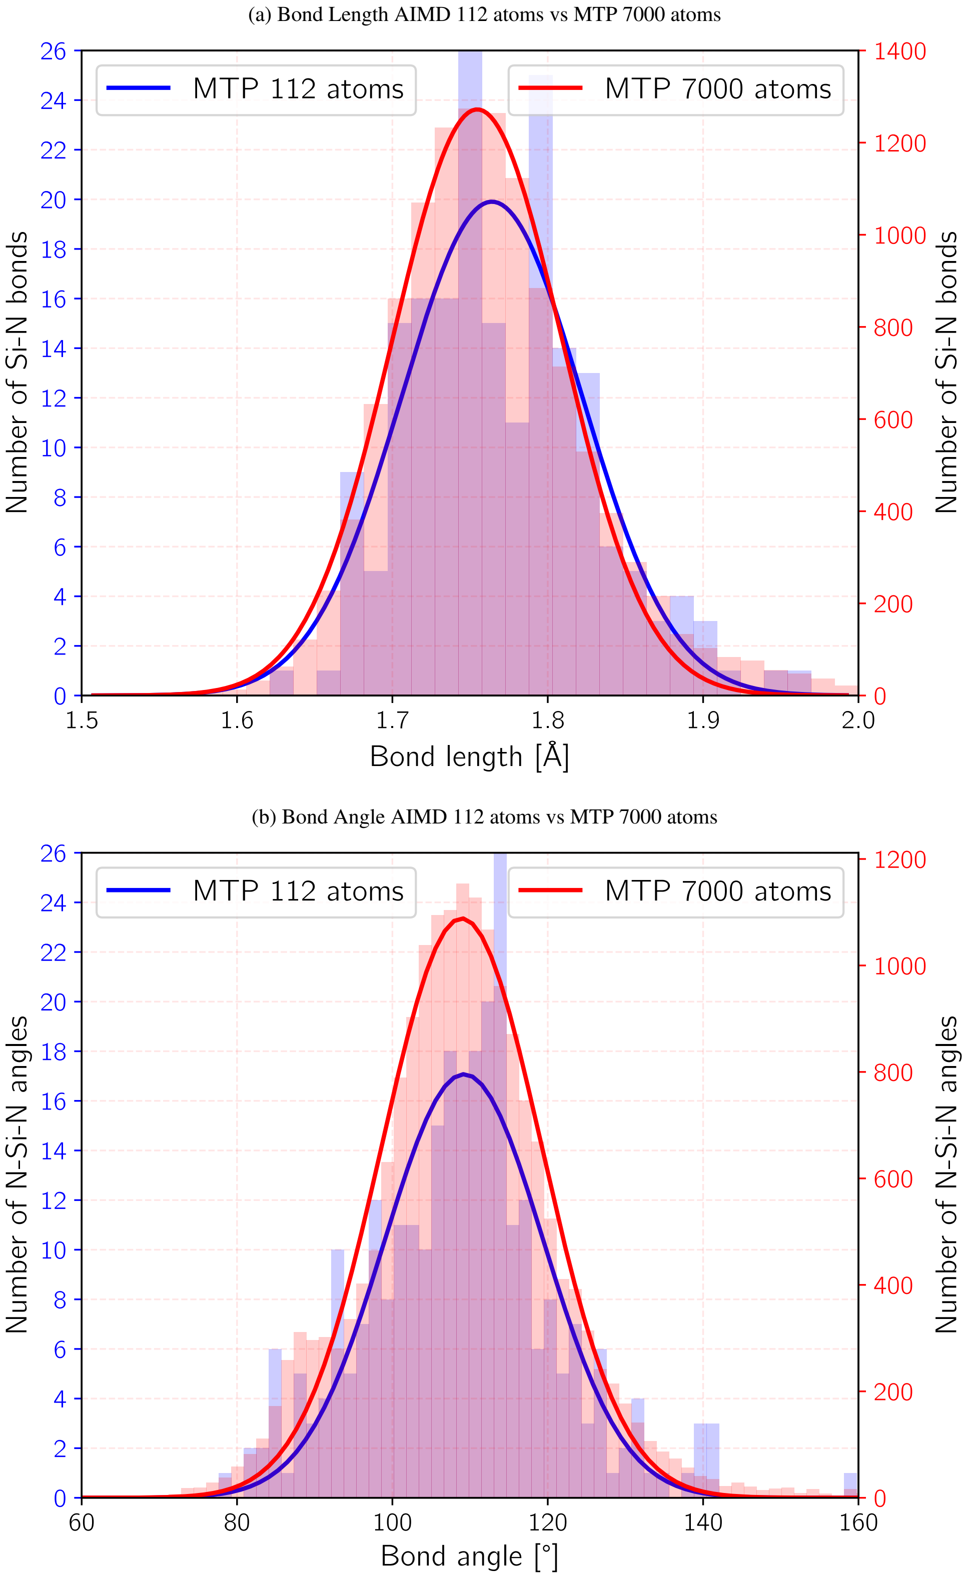


Figure 3: Comparision of (a) bond length distribution and (b) bond angle distribution of MTP small system (112 atoms) to large system (7000 atoms).

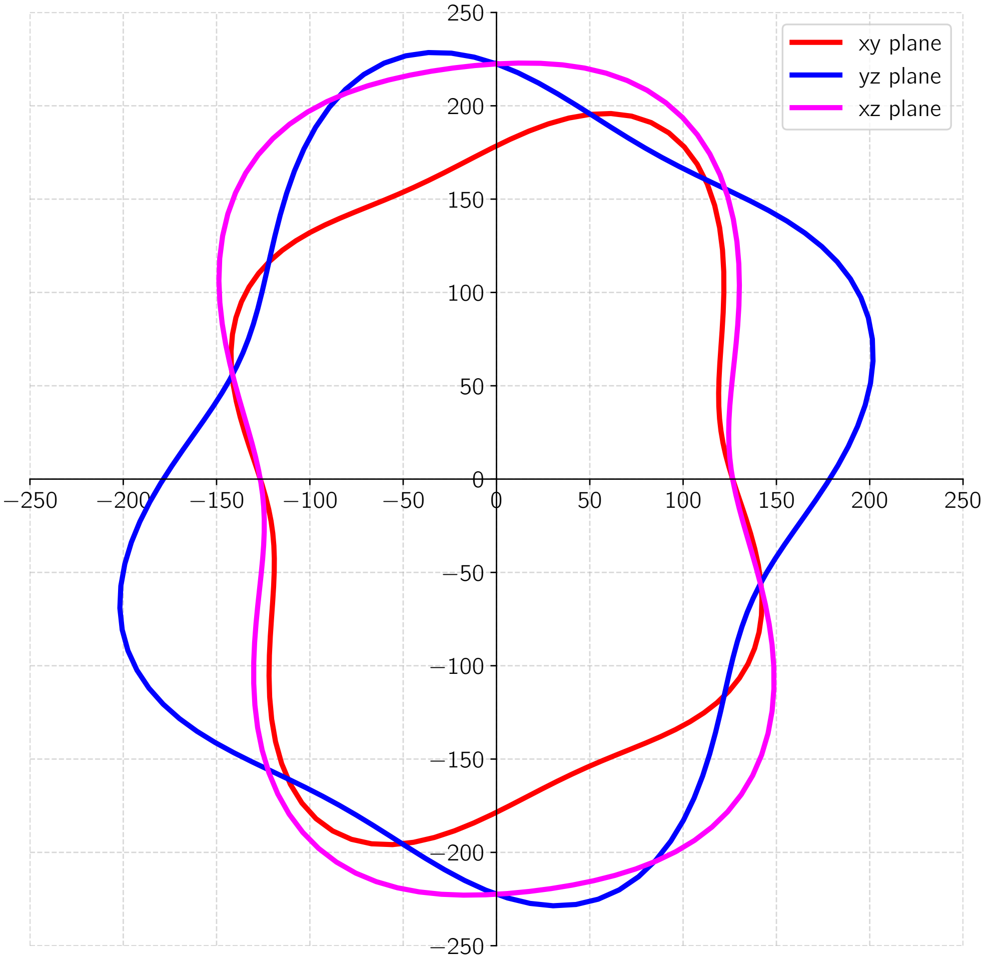


Figure 4: Directional Young's modulus from 0 K calculations plotted along all the directions from GAP with 112 atoms.
